# Supplementary material for: Averaging Spatio-temporal Signals using Optimal Transport and Soft Alignments
Source: arXiv:2203.05813 source file (2022-04-08)
Supplement: Supplementary file 1 [file appendix.tex]

% !TEX root = ../main.tex

% \appendix
